# Supplementary material for: Faithful Chain-of-Thought Reasoning
Source: arXiv:2301.13379 source file (2023-09-20)
Supplement: Supplementary file 1 [file tab_appendix_LM_effect.tex]

\begin{table}[h!]
\centering
\vskip 0.15in
\scalebox{0.8}{
\begin{tabular}{l|rrrr}
    \hline
     \textbf{Exemplars} & GSM8K & Date & SayCan & CLUTRR \\
     \hline
        code-davinci-002 & 71.6 & 80.8 & 89.3 & 58.9 \\
        text-davinci-002 & 62.1 & 76.6 & 79.6 & 43.9 \\
        code-davinci-001 & 26.5 & 43.2 & 66.0 & 23.4 \\
        text-davinci-001 & N/A & N/A & N/A & 17.3 \\
     \hline
\end{tabular}
}
\caption{Accuracy of Faithful COT with different LMs as the Translator, accompanying Figure~\ref{fig:effect_of_LM}. Due to the prompt length limit, \texttt{text-davinci-001} only allows us to run experiments on CLUTRR.}

\label{tab:appendix_LM_effect}
\end{table}
